# Supplementary material for: CONCRETE: Improving Cross-lingual Fact-checking with Cross-lingual Retrieval
Source: arXiv:2209.02071 source file (2022-09-05)
Supplement: Supplementary file 1 [file appendix.tex]

\clearpage
\newpage
\appendix

\section{Dataset Statistics}
We present the detailed statistics of \xict~ in \Cref{tab:dataset_stats}.

\label{sec:dataset_stats}
